# Supplementary material for: In-plane polarization induced ferroelectrovalley coupling in a two-dimensional rare-earth halide
Source: arXiv:2505.17898 source file (2025-05-23)
Supplement: Supplementary file 1 [file sup_mat.pdf]

# Supplemental Materials to
# In-plane polarization induced ferroelectrovalley coupling in a two-dimensional rare-earth halide

Srishti Bhardwaj[1] and T. Maitra[1]

[1] *Department of Physics, Indian Institute of Technology Roorkee, Roorkee - 247667, Uttarakhand, India*

(Dated: May 23, 2025)

## ELECTRONIC BAND STRUCTURES OF 1T AND 2H-$EuCl_2$ MONOLAYERS

In the 1T phase, inversion symmetry is preserved in the monolayer, and hence, no valley splitting is observed. On the other hand, in the 2H-phase, the inversion symmetry is inherently broken in the monolayer and thus, a valley splitting of 47 meV, at K and K′ high-symmetry points, is seen in the 2H-$EuCl_2$ monolayer.

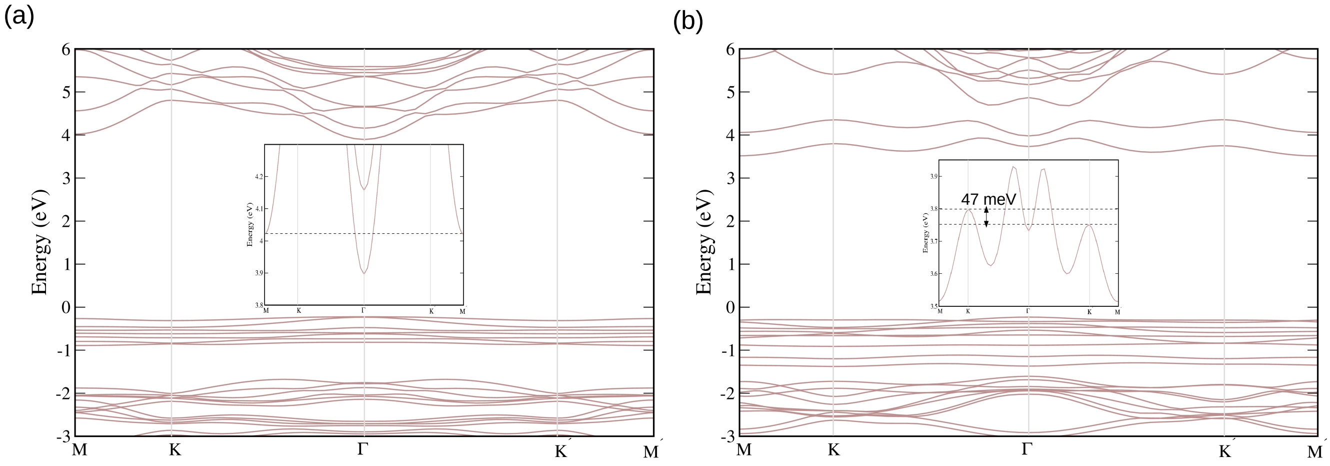


Fig. S1: (a) Electronic band structure with spin-orbit coupling (SOC) for 1T-$EuCl_2$ monolayer and (b) 2H-$EuCl_2$ monolayer. The zoomed-in conduction bands are shown in the insets.

## ORBITAL PROJECTED DOS OF PRISTINE AND $Gd$-SUBSTITUTED 1T $EuCl_2$ MONOLAYER

The valence band in pristine 1T $EuCl_2$ monolayer is formed primarily of half-filled Eu (f) orbitals. In the Gd-substituted monolayer, however, the valence band consists of the extra electron from Gd, and therefore, its orbital composition is mainly Gd (d) and a small part of Eu (d) because of the bond-centered charge ordering (BCO).

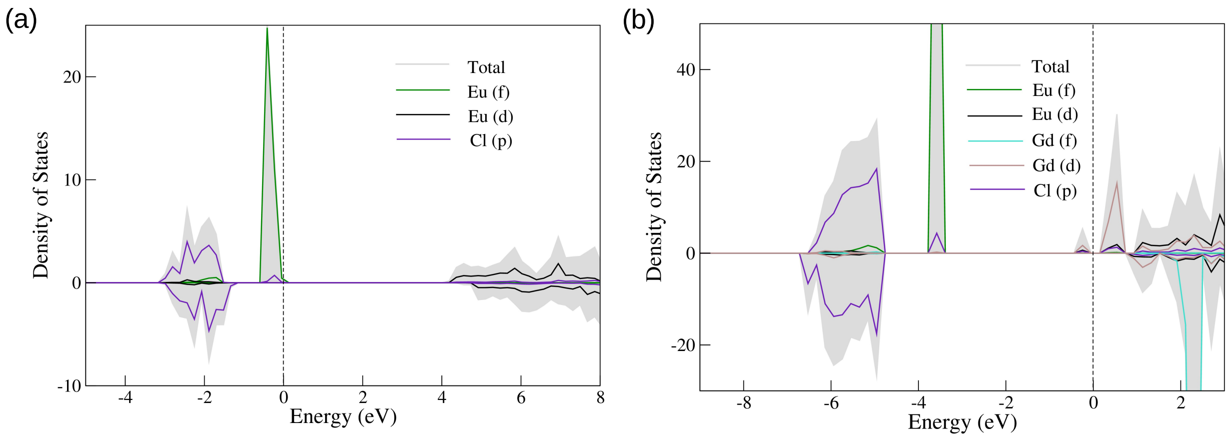


Fig. S2: (a)Orbital projected density of states (DOS) for pristine $EuCl_2$ monolayer. (b) Orbital projected DOS for Gd-substituted 1T-$EuCl_2$ monolayer in FE phase.

## DYNAMIC STABILITY OF AFE AND FE STATES OF $Eu_2GdCl_2$ MONOLAYER

The phonon dispersion spectra of the AFE and FE states of Gd-substituted $EuCl_2$ ML do not show any soft phonon modes, thus indicating the dynamic stability of the monolayer in both phases. (Fig. S3)

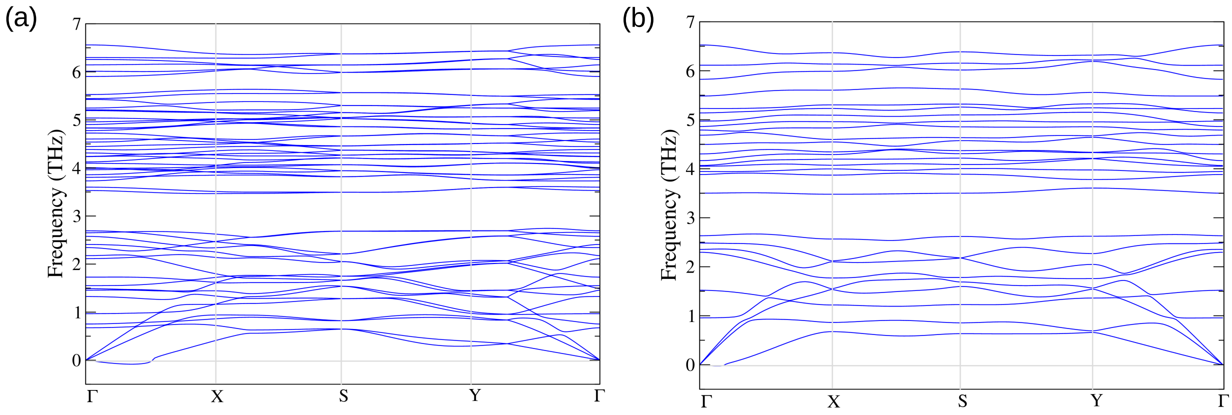


Fig. S3: (a) Phonon dispersion spectrum of anti-ferroelectric structure of Gd-substituted $EuCl_2$ monolayer. (b)Phonon dispersion spectrum of the ferroelectric (FE) counterpart.

## VARIOUS POSSIBLE MAGNETIC CONFIGURATIONS FOR $Eu_2GdCl_2$ MONOLAYER

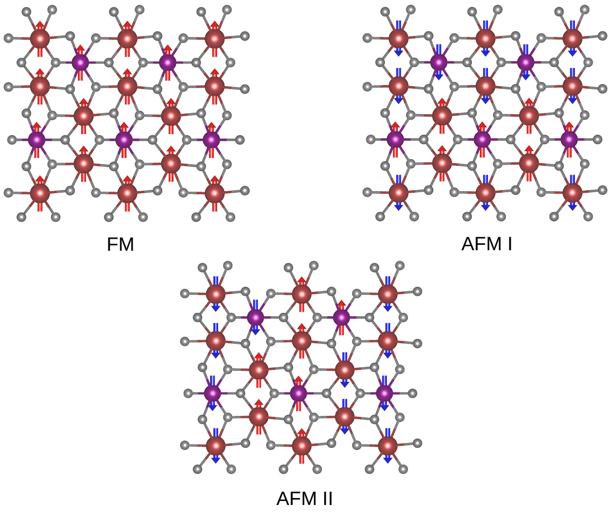


Fig. S4: Magnetic configurations checked for the magnetic ground state of the ferroelectric state of the $Eu_2GdCl_2$ monolayer.

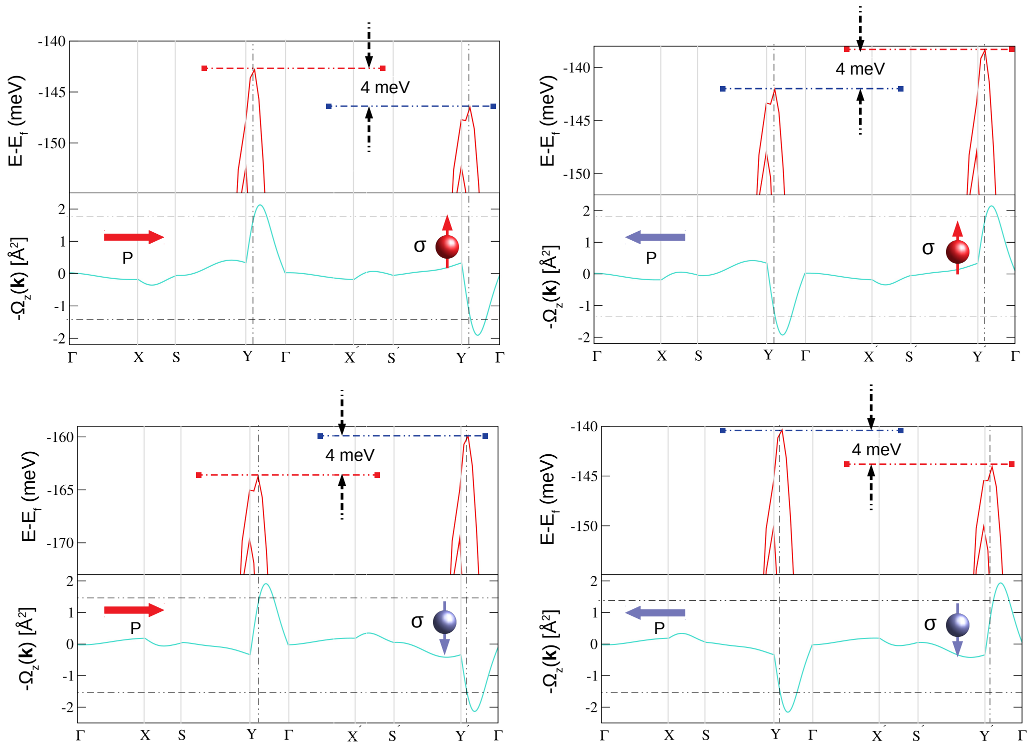


Fig. S5: Zoomed-in electronic band structures shown in Fig.4 to emphasize the valley splitting in the monolayer under 5% tensile strain.
